# Supplementary material for: Learning Deterministic Regular Expressions for the Inference of Schemas from XML Data
Source: arXiv:1004.2372 source file (2010-04-14)
Supplement: Supplementary file 1 [file appendix.tex]

%--------------------------------------------------------------------
% $Id: appendix.tex,v 1.1.1.1 2008-07-18 11:35:17 wouter Exp $
%--------------------------------------------------------------------

\newcommand{\nc}{\newcommand}
\nc{\tin}{\text{in}}
\nc{\out}{\text{out}}
\nc{\sink}{s_{\out}}
\nc{\source}{s_{\tin}}
\nc{\disjunction}{{\sc disjunction}\xspace}
\nc{\concatenation}{{\sc concatenation}\xspace}
\nc{\optional}{{\sc optional}\xspace}
\nc{\selfloop}{{\sc self-loop}\xspace}
\nc{\enabledisjunction}{{\sc enable-disjunction}\xspace}
\nc{\enableoptional}{{\sc enable-optional}\xspace}
\nc{\dm}{\text{dm}\xspace}

\section{Proof of Theorem~\ref{THM:DREG-NOTLEARNABLE}}
\label{sec:proof-theorem-dreg-notlearnable}

 \qed

\section{Proof of Theorem~\ref{THM:KORE-LEARNABLE}}
\label{sec:proof-theorem-kore}

\begin{theorem}
  For every $k$ and $\alphabet$ there exists an algorithm $M$ that learns 
  $\kore(\alphabet)$ from positive data. Furthermore, $M$ runs in time
  polynomial in the size of its input sample $S'$, and in time
  exponential in $k$ and the size of $\alphabet$.
\end{theorem}
\begin{proof}
  \qed

% reduces to membership testing for
%   regular expressions, which can be done in time polynomial in the
%   size of the sample, $k$, and $\car{\alphabet}$.

% any $\koa(\alphabet)$ is
%   of size polynomial in $k$ and $\car{\alphabet}$ and that there thus
%   only exist an exponential number of different $\koas$ over
%   $\alphabet$. Furthermore, testing whether a $\koa(\alphabet)$ is the
%   Glushkov automaton of a $\kore(\alphabet)$ and transforming it into
%   an equivalent $\kore(\alphabet)$ can be done in polynomial time
%   \cite{Caro00}. In conclusion, the set $\mathcal{R}$ of
%   Lemma~\ref{lemma:kore-finiterep} consists of an exponential number
%   of $\kores$ of polynomial size and can be constructed in exponential
%   time, all with respect to $k$ and $\car{\alphabet}$ and independent
%   of the sample size. Imposing the order on the expressions in
%   $\mathcal{R}$ can be done in time polynomial in the size of
%   $\mathcal{R}$ since inclusion of deterministic regular expression
%   can be tested in polynomial time. Finally, we have to test whether a
%   sample is included in a $\kore$ which reduces to membership testing
%   and can be done in time polynomial in the size of the sample, $k$,
%   and $\car{\alphabet}$. This must be done at most once for every $r
%   \in \mathcal{R}$ and hence $M$ runs in time polynomial in the size
%   of the sample and in time exponential in $k$ and
%   $\car{\alphabet}$.\qed
\end{proof}

\section{Proof of Theorem~\ref{THM:KORE-EXP-DATA}}
\label{sec:proof-exp-data}

\begin{theorem}
  Let $\alphabet = \{\sigma_1,\dots, \sigma_n\}$ be an alphabet of
  size $n$, let $r_1 = (\sigma_1 \sigma_2 + \sigma_3 +
  \dots + \sigma_n)^+$, and let $r_2 = \alphabet^+ \sigma_1
  \alphabet^+$. For any algorithm that learns $\dnore{(2n +
    3)}(\alphabet)$ and any sample $S$ that is characteristic for
  $r_1$ or $r_2$ we have $\car{S} \geq \sum_{i=1}^{n}(n-2)^i$.
\end{theorem}

\end{proof}

\renewcommand{\lambda}{\lab}

\section{Proof of Theorem~\ref{THM:TOKORE-SOUND-COMPLETE}}
\label{sec:proof-tokore}

\begin{theorem}
  $\ToSORE$ is sound in the sense that, for every $\koa$ $A$, it
  outputs a (possibly non-deterministic) $\kore$ $r$ with $\lang(A)
  \subseteq \lang(r)$.  It is also complete in the sense that if $A$
  is the Glushkov translation of a deterministic $\kore$ $r'$, then
  $r$ is deterministic and equivalent to $r'$.
\end{theorem}

\begin{proof}

\end{proof}

\section{Simplification rules}
\label{sec:simplification-rules}

Our generated expressions are syntactically simplified using the
following rewrite rules (based on the equivalence relations defined
for the $\ToSORE$ algorithm~\cite{Bex06}):
\begin{eqnarray*}
  r^{*}                     & \rightarrow & r^{+}? \\
  r??                      & \rightarrow & r? \\
  (r^{+})^{+}                & \rightarrow & r^{+} \\
  (r?)^{+}                  & \rightarrow & r^{+}? \\
  (r_1 \cdot r_2) \cdot r_3 & \rightarrow & r_1 \cdot (r_2 \cdot r_3) \\
  r_1 \cdot (r_2 \cdot r_3) & \rightarrow & r_1 \cdot r_2 \cdot r_3 \\
  (r_1? \cdot r_2?)?        & \rightarrow & r_1? \cdot r_2? \\
  (r_1 + r_2) + r_3         & \rightarrow & r_1 + (r_2 + r_3) \\
  r_1 + (r_2 + r_3)         & \rightarrow & r_1 + r_2 + r_3 \\
  (r_1 + r_2^{+})^{+}        & \rightarrow & (r_1 + r_2)^{+} \\
  (r_1^{+} + r_2^{+})        & \rightarrow & (r_1 + r_2)^{+} \\
  r_1 + r_2? & \rightarrow  & (r_1 + r_2)?
\end{eqnarray*}

\newpage

\section{Synthetic regular expressions}
\label{sec:expressions}

\begin{table*}
  \caption{Synthetic regular expressions used for the experiments in
    Section~\ref{sec:synth-target}, derived expressions are only shown
    when not equivalent to the target expression.}
  \begin{tabular}{l|l}
    \textbf{target expression} & \textbf{derived expression} \\ \hline
    $((d a b c) + b + c + e + a)^{*}$ &  \\
    $((b b a) + e + c + a + d)^{+}$ &  \\
    $((b c a b a) + a + d + e + c)^{+}$ &  \\
    $((b a b a c) + e + a + d + c)^{*}$ & $((e? (((b a)^{*} c^{+}) + a + e + d)^{*}) + d + c)^{+}$ \\
    $((b a a c b) + c + e + d + a)^{*}$ & $(a + c + e + (((b a^{+} c b)^{+} + d + e) d^{*}))^{*}$ \\
    $(((((c a b c) + e) a)^{*} b) + a + d)^{+}$ & $(a + d + (((c + e) a)^{*} b^{+}))^{+}$ \\
    $((b? a a b) + c + e + d)^{+}$ &  \\
*    $(((((b a b) + c)^{+} + e)? a) + d)^{+}$ &  \\
    $((d c b a) + e + b + a)^{+}$ &  \\
    $((c b a e) + b + a + d)^{+}$ &  \\
*    $(((b + a) a c b) + e + c + d)^{+}$ &  \\
    $(((c + a) a b c) + d + b + e)^{+}$ &  \\
    $((e c a) + b + c + d)^{*} a b$ &  \\
*    $((((c + d) c a)^{*} a b) + e + b)^{*}$ &  \\
    $(a + e + c + b)^{*} d b a$ &  \\
    $(a + d + b + c)^{*} e b c a$ &  \\
    $(((d a a a b)^{*} e c) + b + c)^{+}$ & $(b + (((d a a^{+} b)^{*} e)? c))^{+}$ \\
    $((((b + d) a)^{+} a b c) + c + e)^{+} + a$ & $((e + c + ((b + d) (a + b)^{+}))^{+} + a)?$ \\
    $((((b + e + d)^{*} a c) + c) a b)?$ &  \\
    $((b b e a) + d + a)^{*} c$ &  \\
    $((d b b e c a a) + c + a)^{*}$ &  \\
    $((d + a + e)^{+} b b c a)?$ &  \\
    $((b + a + c)^{+} d e b a)^{+}$ &  \\
    $(((a d c b) + c + e)^{*} b a)?$ &  \\
    $((((a b c a)^{+} + b)? e)^{+} + d)?$ &  \\
    $((d + a)^{+} c b a) + b + e + c$ &  \\
    $((((a a) + e)^{+} + c) b) + b + d$ &  \\
    $((((d + a)^{*} e a b c b) + c) a)?$ &  \\
    $((((a c) + b + d) e a b) + c)^{*}$ &  \\
    $(((((a^{+} b) + e) b a a)? c)^{+} d c)^{*}$ & $(c + a + a + (d c) + b + (e? b))^{*}$ \\
    $(((d + e)^{+} b a b) + a + c)?$ &  \\
    $((b d c a b c e) + a)^{*}$ &  \\
    $((((b d a) + a)^{+} + c) c b e)^{*}$ &  \\
    $((b^{+} + c + e + d) a a b)^{+}$ &  \\
    $((((e c b)^{+} a) + b)^{+} + d + a)?$ &  \\
    $(((b b d c) + e)^{+} a a a) + c$ &  \\
    $((d + c) e a b a) + b$ &  \\
    $(((b + d) c a)^{+} e c b a)?$ &  \\
    $(((c^{+} + a) a) + d + e + b) b$ &  \\
    $((((c + b) b) + a) c a) + e + d$ &  \\
    $(d c b c a a) + e + a + b$ &  \\
    $(((c + a) a b) + d + f + b + h + i + g + j + e)^{+}$ &  \\
    $(((e + c) e d b a c) + d + j + b + a + g + i + h + f)^{+}$ &  \\
    $(((j b a) + c + i + h + b + f + e + d)^{+} + a + g)?$ &  \\
    $((((g + i) h)^{+} a b) + e + j + b + a + f + d + c)^{*}$ &  \\
    $((((g b) + h + c) a f) + a + e + j + d + i)^{+} + b$ &  \\
    $(((((d e j b) + g) a d c) + i + c + f + b + e + h)^{*} a)^{+}$ &  \\
    $((((j + a) a c e b e d) + h + c + d + b + g + i)^{+} + f)?$ &  \\
    $((f b a) + b + j + c + h + i)^{+} + d + e + g + a$ &  \\
    $((f i g j b a) + c + d + b + a + h + e)^{+}$ &  
  \end{tabular}
\end{table*}
\addtocounter{table}{-1}
\begin{table*}
  \caption{Continued}
  \begin{tabular}{l|l}
    \textbf{target expression} & \textbf{derived expression} \\ \hline
    $(((i + e) f a b j) + d + h + a + b + g)^{+} c$ &  \\
    $(((((i h a a j) + d)^{+} + g) b) + e + b + f + c)^{+}$ &  \\
    $((g + b + e + f + i + d)^{*} a b a) + h + j + c$ &  \\
    $((b a g b f e i d) + c + a + j + h)^{*}$ &  \\
    $((g d a b) + a + i + c + j + e + f)^{+} h b$ &  \\
    $((h^{*} c d f a) + j + e + g + b + i)^{*} a b$ &  \\
    $((((a? d)^{+} b a) + h + g + e + c)^{+} + j + i + b)? f$ &  \\
    $((((e a b h) + d + j + c + b)^{+} f) + a + g + i)?$ &  \\
    $(((e c g e c d) + b + d + a + j + f)^{*} i h a b a)^{*}$ &  \\
    $(((c + b) a b) + d + i + a)^{+} + j + g + f + e + h$ &  \\
    $((((j h b f e d c)^{*} i)^{*} g a) + a + d + b)^{*} e c$ &  \\
    $(((b + h + a) c b d g j a) + e + f + i)^{+}$ &  \\
    $((h + j + e + g + c + f + d)^{*} a i d e c a b b)?$ &  \\
    $((((h + b + c + j + f)^{+} + e)? a a i d b) + g)?$ &  \\
    $(((i + e + a + c + h)^{+} + g + d)? b b a f j)^{+}$ &  \\
    $(((((c b i) + a + j) g d a) + f + b + e)? h)^{+}$ &  \\
    $((((f + c + h + b)^{*} e b d) + j) a i g a)^{+}$ &  \\
    $(((j b e c) + e + d + i)^{+} + h + b)? a g d a a c f$ &  \\
    $(((((f a) + d)^{*} c)^{+} i d g j c a a e e b) + b + h)^{+}$ & $(h + (((((f a) + d)^{*} c)^{+} i d g j c a^{+} e e)? b^{+}))^{+}$ \\
    $((((a d a) + j)^{+} d c e h f b e b g) + c + i)^{*}$ &  \\
    $((((e + h)^{+} + c) a b) + d + b + j + a + i + g + f)?$ & $(((((h + e + e)^{+} + c)? a)? b) + a + d + f + g + i + j)?$ \\
    $((((((b + f + e + h + i) e) + j)^{+} a c d)? g b) + c + d) a$ &  \\
    $(((d^{+} + h + j)? g)^{+} + c + i) a a e b b f$ &  \\
    $(((c + a + f + j)^{+} + g)? b d)^{*} h e a a d b e c i$ & $((b d) + g + c + f + j + a + (h e a))^{*} d b e c i$ \\
    $(((((b + a + j) d) + e + d)^{+} f b a g c i e) + c + h)?$ &  \\
    $((((e d g i c b d f a c) + j + a) e)^{+} + b + h)?$ &  \\
    $((d + j)^{+} g i a b f a d e b c)^{+} + a + c + h + e$ &  \\
    $((((((h + d + c)? e c e) + g + i) b f a d a) + b + a) j)^{*}$ &  \\
    $(((((f? b a)^{*} e d e) + g)^{*} c d j a h c b) + i)?$ &  \\
    $((((b a b) + c + i + f + e + j + a) a c e d d) + h)^{*} g$ &  \\
    $((b e c h g a i f b d) + j) a$ &  \\
    $(((((c^{+} a) + j) c e d f b) + g + e + d) b i a a)^{+} + h$ &  \\
    $(a + b + f) a e c d d b c e h j i g$ &  \\
    $((g + a + e + j + f) b a) + d + b + c + i + h$ &  \\
    $((b b)^{+} e d c j h f g)? a a i$ &  \\
    $(((k? j g h a d f c e l i f c j b h o m) + b + g + a + e + i + n)^{+} + d)?$ &  \\
    $((a e d o a d e n h d b c i) + h + k + m + j + g + b)^{*} f c c g e l b i f j a$ &  \\
    $((a + k + f + c + m + e)^{+} b d i e c l b o n j g d a)^{*} h$ &  \\
    $(l + c + d + m + n)^{*} a o j a h b e g c b f i d k e$ &  \\
    $(a^{+} + f + d + o + g + n + h + c + b + j + i + e) k e a c d l b m$ &  \\
    $(((a? c l f h a b g d) + b + n + o) i e d j c e m)^{*} k$ &  \\
    $(((k + f + o + a + j)? e d h l d f h n g i c j m a b)? c i e)^{*} b g$ &  \\
    $(((e a)^{*} d b) + b + a + c)^{+}$ &  \\
    $(((a d a b) + b + e)^{+} + c)?$ &  \\
    $((c^{+} b b a) + a + d)? e$ &  \\
    $((d e b a b) + c)^{*} a$ &  \\
    $(((((d b e)^{*} c f) + j) h a c) + b + i)^{*} g a d$ &  \\
    $(((e a)^{*} d b) + b + a + c)^{+}$ &  \\
    $(((a d a b) + b + e)^{+} + c)?$ &  \\
    $((c^{+} b b a) + a + d)? e$ &  \\
    $((d e b a b) + c)^{*} a$ &  \\
    $(((((d b e)^{*} c f) + j) h a c) + b + i)^{*} g a d$ &  \\
    $(((e^{*} h c d a f e g a i f g c d b j b)^{*} i n h j a l e)^{+} + o + b + d + c + k + m)?$ & $(((e^{*} h c d a f e g a i f g c d b j b)^{*} i n h j a l e)^{+} + o + b + d + c + k + m)?$ \\
    $((((((d b e h c l f) + j)? b a)? e d g) + c + i)^{+} + o + n + m + a + k)?$ & $((((((d b e h c l f) + j)? b a)? e d g) + c + i)^{+} + o + n + m + a + k)?$ \\
  \end{tabular}
\end{table*}

%%% Local Variables: 
%%% mode: latex
%%% TeX-master: "pomm"
%%% End: 

%%% Local Variables: 
%%% mode: latex
%%% TeX-master: "pomm"
%%% End: 
